# Supplementary material for: Train Small, Model Big: Scalable Physics Simulators via Reduced Order Modeling and Domain Decomposition
Source: arXiv:2401.10245 source file (2023-12-06)
Supplement: Supplementary file 1 [file appendix.tex]

\section{Verification of the Stokes flow equation solver}\label{sec:stokes-mms}
We consider a manufactured solution $\tbq = (\tilde{\bu}, \tilde{p})$ over a unit square domain $\Omega = [0, 1]^2$,
\begin{subequations}\label{eq:stokes-mms-sol}
    \begin{equation}
        \tilde{\bu}=
        \begin{pmatrix}
            \cos(x_1)\sin(x_2)\\
            -\sin(x_1)\cos(x_2)
        \end{pmatrix}
    \end{equation}
    \begin{equation}
        \tilde{p} = 2\nu\sin(x_1)\sin(x_2).
    \end{equation}
\end{subequations}
The manufactured solution must satisfy the Stokes flow equation (\ref{eq:stokes-gov}) with a forcing,
\begin{subequations}\label{eq:stokes-mms}
    \begin{equation}
        -\nu\nabla^2 \tilde{\bu} + \nabla\tilde{p} =
        \begin{pmatrix}
            4\nu\cos(x_1)\sin(x_2) \\ 0
        \end{pmatrix}
    \end{equation}
    \begin{equation}
        \nabla\cdot\tilde{\bu} = 0.
    \end{equation}
\end{subequations}
Dirichlet boundary condition is set for $\tilde{\bu}$ on all boundaries.
(\ref{eq:stokes-mms}) is discretized as described in Section~\ref{subsec:stokes-dg}, with $M=1$.
\begin{figure}[tbhp]
    \input{stokes_mms.tex}
    \caption{
        Performance of the FOM Stokes flow solver with preconditioner:
        (a) scaling of the computation time;
        and (b) relative error with respect to (\ref{eq:stokes-mms-sol}).
    }
    \label{fig:stokes-mms}
\end{figure}
Figure~\ref{fig:stokes-mms} shows the scaling and convergence of the MINRES solver with relative tolerance of $10^{-10}$.
With preconditioner (\ref{eq:stokes-prec}),
the computation time scales linearly with the size of the system in Figure~\ref{fig:stokes-mms}~(a),
as reported in~\cite{Elman2014}.
The relative error shows the expected convergence behavior with $s=1$ in (\ref{eq:stokes-Qms}).
